# Supplementary material for: Discovery of fully efficient fault indicators along a data-based diagnosis process
Source: arXiv:2609.28087 source file (2026-09-23)
Supplement: Supplementary file 1 [file appendices.tex]

\appendix

\begin{comment}
\section{Log loss to accuracy conversion}
\label{apdx:log_loss}
%In order to avoid applying the logarithm function to 0, the \textproc{log\_loss} function in $gplearn$ uses a technique known as clipping, which consists in replacing probabilities equal to 0 with $10^{-15}$. Given that DT4X uses \textproc{log\_loss} with a decision function that can only return 0 or 1, that meant that the \textproc{log\_loss} of a sample can only take the values \{$10^{-15}, 1-10^{-15}$\}. The total log-loss is thus a linear transformation of the number of misclassified samples. From this, we can derive:
%\[log\_loss < 1 \Leftrightarrow (1 - accuracy)\times 34.54 < 1\]
%\[\Leftrightarrow accuracy > 0.97\]
%This value corresponds to the minimum target-class separation quality required for an expression to be considered satisfactory by the DT4X fitness function.

The \textproc{log\_loss} function in \texttt{gplearn} cannot operate on probabilities equal to~0, since 
$\log(0)$ is undefined. To avoid this issue, the implementation uses \emph{clipping}, replacing 
predicted probabilities equal to~0 with $10^{-15}$, and probabilities equal to~1 with 
$1 - 10^{-15}$. In DT4X, the decision function outputs only $0$ or $1$, so after clipping, the 
effective probabilities passed to \textproc{log\_loss} are restricted to the set 
$\{10^{-15},\, 1 - 10^{-15}\}$. As a consequence, the log-loss of a sample takes only two 
possible values, depending solely on whether the sample is correctly or incorrectly classified.

For a misclassified sample, the clipped probability is $p = 10^{-15}$, leading to a log-loss of
\[
    -\log(10^{-15}) = 15 \log(10) \approx 34.54.
\]
For a correctly classified sample, the clipped probability is $p = 1 - 10^{-15}$, for which
\[
    -\log(1 - 10^{-15}) \approx 10^{-15},
\]
a negligible value. Thus, the total log-loss becomes essentially proportional to the number of 
misclassified samples. Let $N$ be the total number of samples and $N_{\text{incorrect}}$ the number of 
misclassified ones. The accuracy is defined as
\[
    \text{accuracy} = 1 - \frac{N_{\text{incorrect}}}{N}.
\]
Since each misclassified sample contributes approximately $34.54$ to the log-loss, we obtain
\[
    \text{log\_loss} \approx (1 - \text{accuracy}) \times 34.54.
\]
Hence,
\[
    \text{log\_loss} < 1
    \;\;\Leftrightarrow\;\;
    (1 - \text{accuracy}) \times 34.54 < 1
    \;\;\Leftrightarrow\;\;
    \text{accuracy} > 0.97.
\]
This threshold corresponds to the minimum target-class separation quality required for an expression
to be considered satisfactory by the DT4X fitness function.
\end{comment}

\section{Hyperparameters}
\label{apdx:hyperparam}
\begin{table}[htpb]
    \resizebox{\columnwidth}{!}{%
    \begin{tabular}{|c|c|}\hline
         \textbf{System} & \textbf{Hyperparameters} \\\hline
         sf\_polybox & \makecell[l]{
            parsimony\_coefficient=0.06, max\_depth=2,\\
            arr\_perf\_threshold=0.97, number\_of\_generations=20,\\
            population\_size=20000, function\_set=\{add, sub, mul\}} \\\hline
         sf\_subtractor & \makecell[l]{
            parsimony\_coefficient=0.05, max\_depth=2,\\
            arr\_perf\_threshold=0.97, population\_size=10000,\\
            function\_set=\{xor\_func, not\_func, or\_func, and\_func\}} \\\hline
         sw\_water\_tanks & \makecell[l]{
            epsilon=0.03, parsimony\_coefficient=0.0002, max\_depth=6,\\
            relevant\_proportion\_of\_individuals=0.0001,\\
            number\_of\_generations=35, function\_set=\{add, sub, mul,\\
            div\_custom, sqrt\_custom, sqr\_custom\}} \\\hline
         steam\_superheater\_42 & \makecell[l]{
            epsilon=0.01, parsimony\_coefficient=0.0005, max\_depth=6,\\
            relevant\_proportion\_of\_individuals=0.01,\\
            number\_of\_generations=40, population\_size=5000,\\
            function\_set=\{add, sub, mul, div\_custom\}} \\\hline
    \end{tabular}
    }
    \caption{Hyperparameters per system.}
    \label{tab:hyperparameters}
\end{table}

\section{Tree and confusion matrix comparison}
\label{apdx:tree-comparision}

As mentioned in Sec.~\ref{sec:results}, the performance metrics do not tell the whole story, with the confusion matrices and tree structures revealing extra insights into the comparison of the algorithms.

\begin{figure}[htpb]]
  \includegraphics[width=0.8\linewidth]{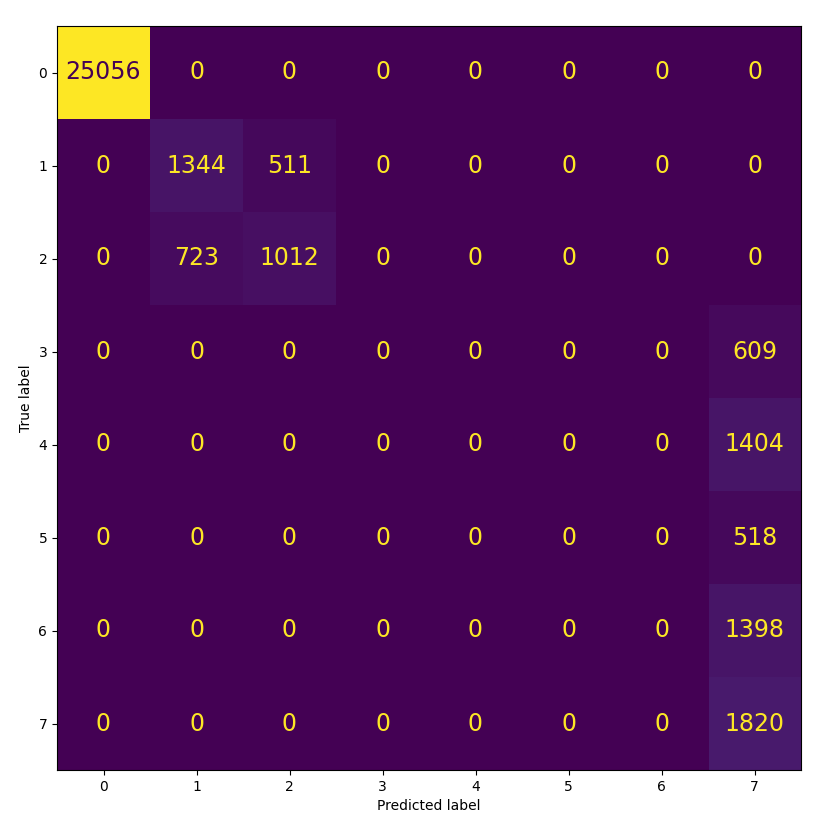}
\caption{DT4X confusion matrix on the sf\_subtractor dataset.}
\label{fig:cm_DT4X}
\end{figure}

Fig.~\ref{fig:cm_DT4X} shows that DT4X does not properly differentiate between classes 1 and 2, with a significant number of both false positives and false negatives of either class being tagged as the other. 
This changes however for DT4X+, where, as seen in Fig~\ref{fig:cm_DT4X+}, a subset of class 1 is correctly identified, with no class 1 false positives, while the predicted class 2 still contains class 1 individuals.

\begin{figure}[H]
  \includegraphics[width=0.8\linewidth]{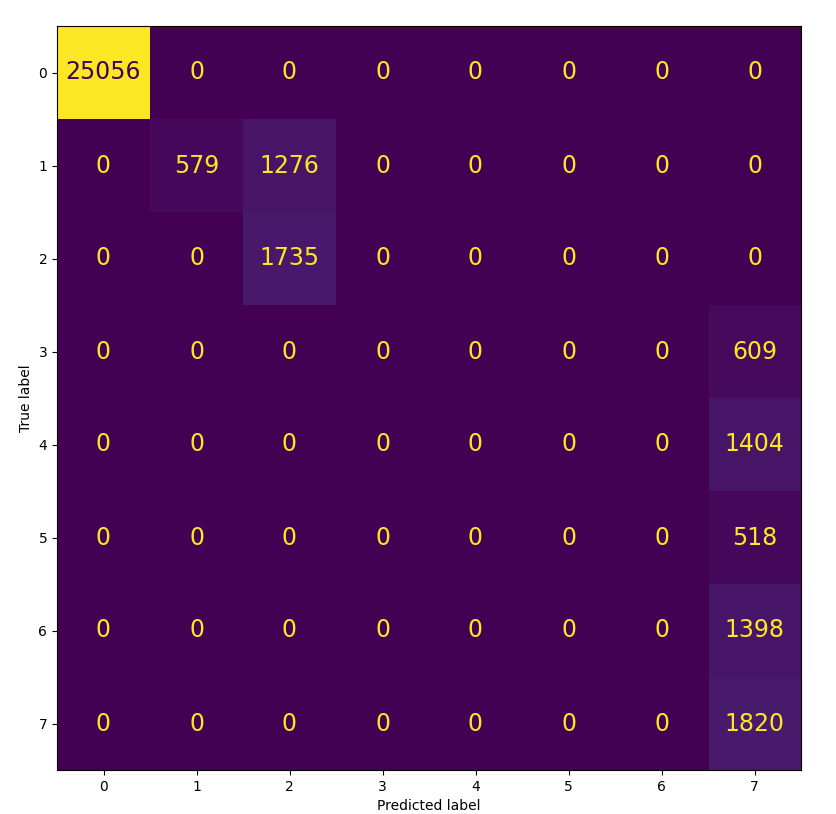}
\caption{DT4X+ confusion matrix on the sf\_subtractor dataset.}
\label{fig:cm_DT4X+}
\end{figure}

Furthermore, when looking at the tree structure in Fig.~\ref{fig:tree_DT4X}, we can see that the expression at Node 0 does not give any information about class 2, with its samples ending up in both Node 1 and Node 2. This is not the case with the tree generated by DT4X+ as seen in Fig.~\ref{fig:tree_DT4X+}, where no class 2 samples can be found in Node 2, meaning that the fault indicator found by DT4X+ for Node 0 is more useful than the one found by DT4X.

While the trees generated by either algorithm for the sw\_water\_tanks dataset are too large to be shown here in their entirety, Fig.~\ref{fig:DT4X_top} and Fig.~\ref{fig:DT4X+_top} show the top split of respectively, DT4X and DT4X+. On the one hand, as shown in Fig.~\ref{fig:DT4X_top}, DT4X splits most classes into both nodes only really providing information about classes 0, 1, 2 and 3, while the other classes are split among Node 1 and Node 2. On the other hand, Fig.~\ref{fig:DT4X+_top} shows that DT4X+ isolated each of the classes into one of the two nodes, with only classes 0, 3, 5 and 10 having a presence in both Node 1 and 2, though still having a very significant majority in one of the two nodes.

\begin{figure}[h]
    \centering
\tikzset{every tree node/.style={minimum width=2em,draw,rectangle},
     blank/.style={draw=none},
     edge from parent/.style=
     {draw, edge from parent path={(\tikzparentnode) -- (\tikzchildnode)}},
     level distance=6.5cm}
\resizebox{0.6\columnwidth}{!}{%
\begin{tikzpicture} 
\Tree
[.\makecell{Node : 0\\$(-d\_y4 + (y3 - y4)^4/y3)^4$\\0 vs 8\\class 0 (Faultless) : 91024 \\class 1 (f\_a) : 22553 \\class 2 (f\_hl) : 21825 \\class 3 (f\_h2) : 21715 \\class 4 (f\_f1) : 21871 \\class 5 (f\_f2) : 21100 \\class 6 (f\_11) : 20472 \\class 7 (f\_12) : 21831\\ class 8 (f\_l3) : 23535\\ class 9 (f\_cl) : 21157\\ class 10 (f\_c2) : 21005}
    [.\makecell{Node : 1\\ class 0 (Faultless) : 91020\\ class 1 (f\_a) : 22553\\ class 2 (f\_hl) : 21825\\ class 3 (f\_h2) : 21715\\ class 4 (f\_f1) : 2866\\ class 5 (f\_f2) : 8706\\ class 6 (f\_l1) : 19304\\ class 7 (f\_l2) : 791\\ class 9 (f\_c1) : 20412\\ class 10 (f\_c2) : 15791} ]
    [.\makecell{Node: 2\\ class 4 (f\_f1) : 19005\\ class 5 (f\_f2) : 12394\\class 6 (f\_l1) : 1168\\class 7 (f\_l2) : 21040\\ class 8 (f\_13) : 23535\\class 9 (f\_c1) : 745\\ class 10 (f\_c2) : 5214} ] 
]
\end{tikzpicture}
    }
    \caption{Top split of the DT4X tree for sw\_water\_tanks.}
    \label{fig:DT4X_top}
\end{figure}


\begin{figure}[h]
    \centering
\tikzset{every tree node/.style={minimum width=2em,draw,rectangle},
     blank/.style={draw=none},
     edge from parent/.style=
     {draw, edge from parent path={(\tikzparentnode) -- (\tikzchildnode)}},
     level distance=6.5cm}
\resizebox{0.8\columnwidth}{!}{%
\begin{tikzpicture} 
\Tree
[.\makecell{Node : 0\\$(d\_y2/d\_y4 + d\_y4*y4^3/y2 - y3^{0.25})/(d\_y2^2/d\_y4^2 + u\_ref + y4^6/y2^2)$\\0 vs 8\\class 0 (Faultless) : 91024 \\class 1 (f\_a) : 22553 \\class 2 (f\_h1) : 21825 \\class 3 (f\_h2) : 21715 \\class 4 (f\_f1) : 21871 \\class 5 (f\_f2) : 21100 \\class 6 (f\_l1) : 20472 \\class 7 (f\_l2) : 21831\\ class 8 (f\_l3) : 23535\\ class 9 (f\_c1) : 21157\\ class 10 (f\_c2) : 21005}
    [.\makecell{Node : 1\\ class 0 (Faultless) : 91020\\ class 1 (f\_a) : 22553\\ class 2 (f\_h1) : 21825\\ class 3 (f\_h2) : 21714\\ class 4 (f\_f1) : 21871\\ class 5 (f\_f2) : 21048\\ class 6 (f\_l1) : 20472\\ class 7 (f\_l2) : 21831\\ class 9 (f\_c1) : 21157\\ class 10 (f\_c2) : 1} ]
    [.\makecell{Node: 2\\ class 0 (Faultless) : 4\\ class 3 (f\_h2) : 1\\ class 5 (f\_f2) : 52\\ class 8 (f\_l3) : 23535\\ class 10 (f\_c2) : 21004} ] 
]
\end{tikzpicture}
    }
    \caption{Top split of the DT4X+ tree for sw\_water\_tanks.}
    \label{fig:DT4X+_top}
\end{figure}

\begin{figure*}
\centering
  \includegraphics[width=0.8\textwidth]{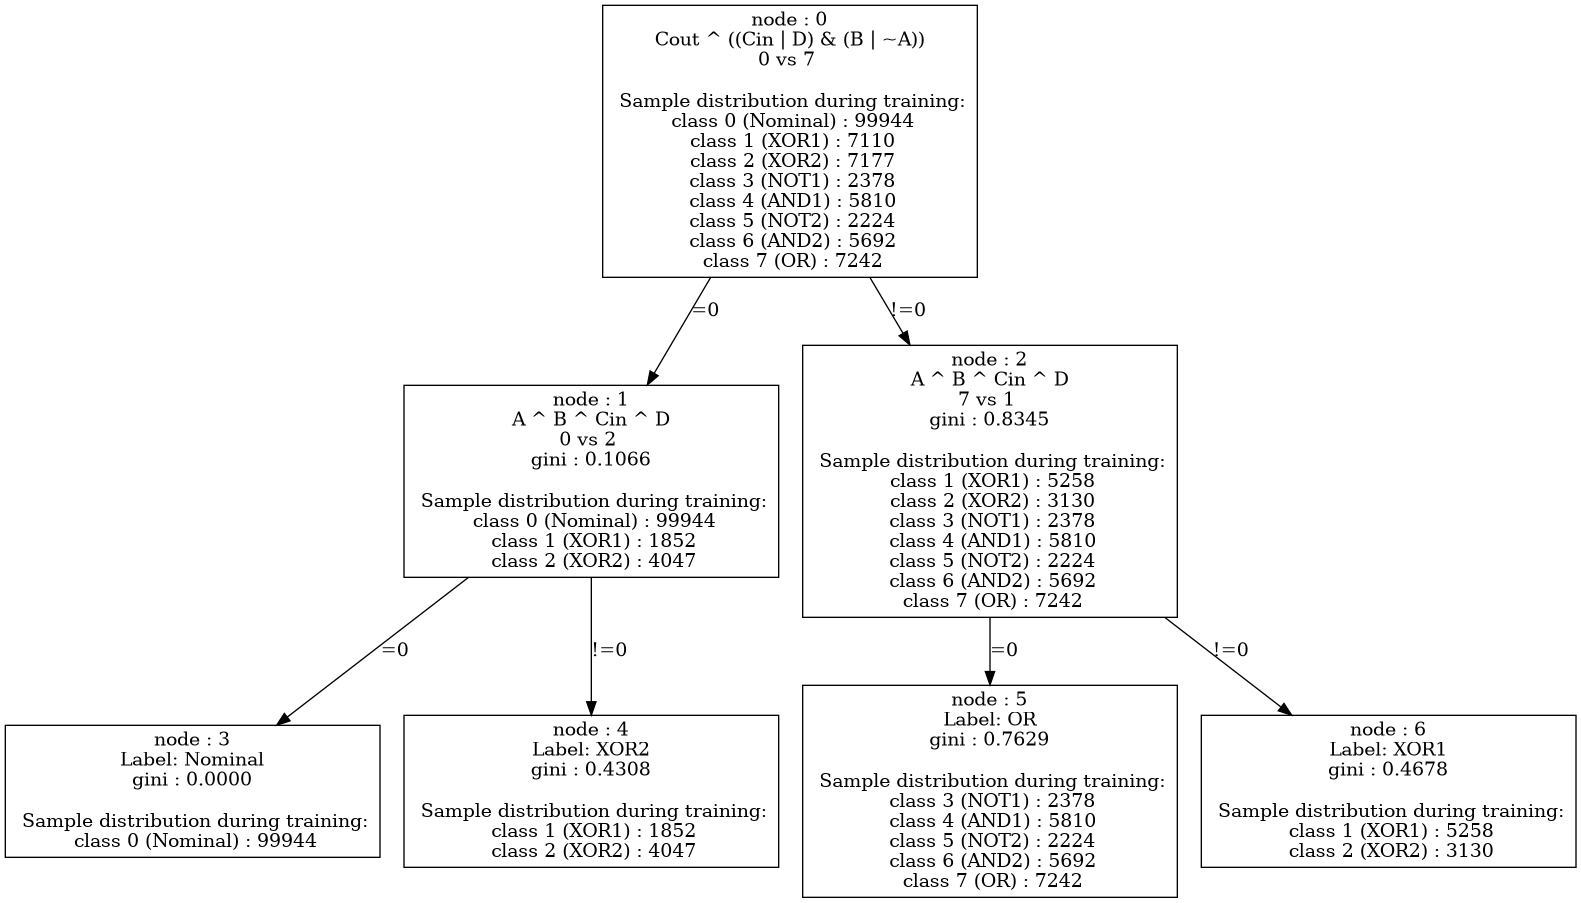}
  \caption{DT4X tree for the sf\_subtractor dataset.}
\label{fig:tree_DT4X}
\end{figure*}

\begin{figure*}
    \centering
    \includegraphics[width=0.8\textwidth]{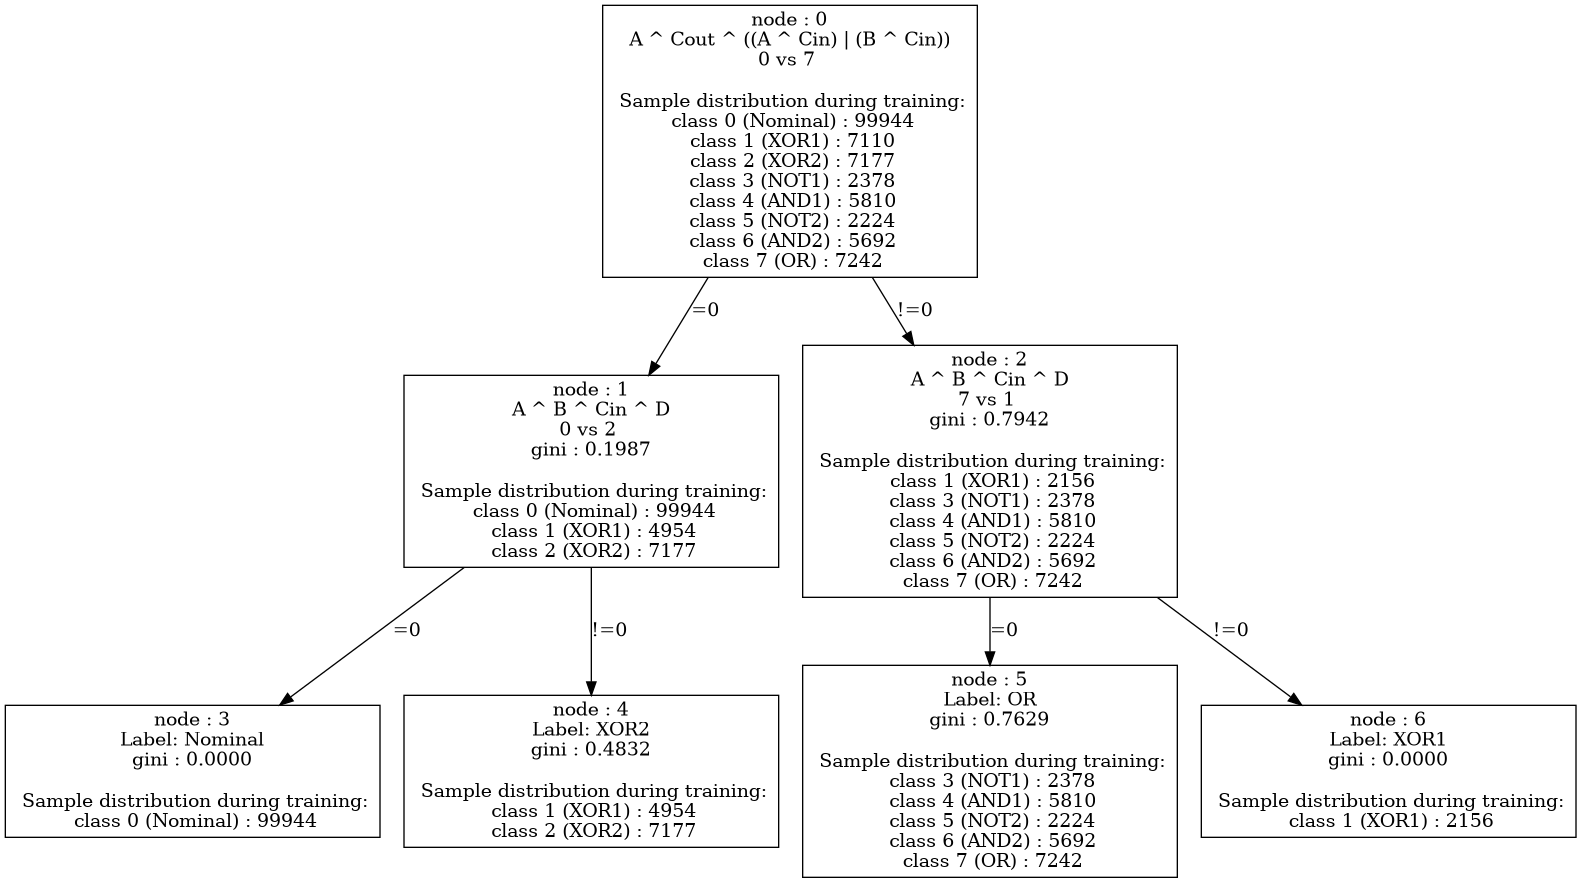}
    \caption{DT4X+ tree for the sf\_subtractor dataset.}
    \label{fig:tree_DT4X+}
\end{figure*}
